# Supplementary material for: Density-gradient-free variable in exchange-correlation functionals for detecting inhomogeneities in the electron density
Source: arXiv:1808.08887 ancillary file (2018-12-23)
Supplement: Supplementary file 1 [file Supplemental_Material.pdf]

# Supplemental Material for
# Density-gradient-free variable in exchange-correlation functionals for detecting inhomogeneities in the electron density

Fabien Tran and Peter Blaha
*Institute of Materials Chemistry, Vienna University of Technology,*
*Getreidemarkt 9/165-TC, A-1060 Vienna, Austria*

TABLE S1. Equilibrium lattice constant $a_0$ (in Å) of 44 solids. All results were obtained non-self-consistently using PBE orbitals/density. The space group number is indicated in parenthesis.

| Solid | Expt. | LDA | PBE | PBEsol | PBE$u$(PBE) | PBE$u$(PBEsol) | PBE$u$(0.10,0.02) |
|---|---|---|---|---|---|---|---|
| C (227) | 3.553 | 3.536 | 3.575 | 3.557 | 3.563 | 3.550 | 3.550 |
| Si (227) | 5.412 | 5.402 | 5.471 | 5.434 | 5.434 | 5.423 | 5.416 |
| Ge (227) | 5.641 | 5.626 | 5.764 | 5.678 | 5.638 | 5.633 | 5.628 |
| Sn (227) | 6.477 | 6.478 | 6.657 | 6.543 | 6.445 | 6.474 | 6.452 |
| SiC (216) | 4.346 | 4.335 | 4.385 | 4.362 | 4.372 | 4.358 | 4.351 |
| BN (216) | 3.592 | 3.585 | 3.628 | 3.610 | 3.619 | 3.602 | 3.602 |
| BP (216) | 4.525 | 4.493 | 4.550 | 4.522 | 4.529 | 4.515 | 4.510 |
| AlN (216) | 4.368 | 4.349 | 4.408 | 4.383 | 4.384 | 4.372 | 4.364 |
| AlP (216) | 5.451 | 5.440 | 5.513 | 5.476 | 5.478 | 5.463 | 5.459 |
| AlAs (216) | 5.649 | 5.636 | 5.735 | 5.681 | 5.656 | 5.650 | 5.646 |
| GaN (216) | 4.509 | 4.464 | 4.553 | 4.505 | 4.478 | 4.470 | 4.472 |
| GaP (216) | 5.439 | 5.395 | 5.508 | 5.442 | 5.414 | 5.402 | 5.406 |
| GaAs (216) | 5.640 | 5.607 | 5.749 | 5.663 | 5.630 | 5.618 | 5.616 |
| InP (216) | 5.858 | 5.830 | 5.959 | 5.880 | 5.829 | 5.828 | 5.833 |
| InAs (216) | 6.047 | 6.028 | 6.185 | 6.087 | 6.028 | 6.028 | 6.027 |
| InSb (216) | 6.473 | 6.452 | 6.635 | 6.520 | 6.434 | 6.449 | 6.439 |
| LiH (225) | 3.979 | 3.914 | 4.008 | 3.981 | 4.006 | 3.971 | 3.968 |
| LiF (225) | 3.972 | 3.915 | 4.069 | 4.008 | 4.127 | 4.005 | 4.014 |
| LiCl (225) | 5.070 | 4.966 | 5.151 | 5.065 | 5.100 | 5.007 | 5.058 |
| NaF (225) | 4.582 | 4.510 | 4.705 | 4.633 | 4.657 | 4.574 | 4.580 |
| NaCl (225) | 5.569 | 5.468 | 5.699 | 5.607 | 5.614 | 5.514 | 5.558 |
| MgO (225) | 4.189 | 4.167 | 4.258 | 4.220 | 4.229 | 4.199 | 4.197 |
| Li (229) | 3.443 | 3.365 | 3.436 | 3.434 | 3.459 | 3.448 | 3.420 |
| Na (229) | 4.205 | 4.054 | 4.199 | 4.171 | 4.147 | 4.133 | 4.101 |
| Al (225) | 4.022 | 3.983 | 4.041 | 4.015 | 4.018 | 4.008 | 4.000 |
| K (229) | 5.246 | 5.044 | 5.283 | 5.215 | 5.329 | 5.199 | 5.169 |
| Ca (225) | 5.559 | 5.334 | 5.527 | 5.456 | 5.659 | 5.476 | 5.491 |
| Rb (229) | 5.629 | 5.373 | 5.671 | 5.569 | 5.669 | 5.511 | 5.513 |
| Sr (225) | 6.059 | 5.785 | 6.024 | 5.917 | 6.126 | 5.894 | 5.966 |
| Cs (229) | 6.043 | 5.754 | 6.161 | 6.010 | 6.381 | 5.986 | 6.067 |
| Ba (229) | 4.994 | 4.752 | 5.021 | 4.880 | 5.259 | 4.829 | 5.015 |
| V (229) | 3.023 | 2.927 | 2.998 | 2.960 | 2.932 | 2.927 | 2.932 |
| Ni (225) | 3.510 | 3.422 | 3.517 | 3.462 | 3.470 | 3.434 | 3.449 |
| Cu (225) | 3.599 | 3.522 | 3.632 | 3.567 | 3.627 | 3.550 | 3.576 |
| Nb (229) | 3.300 | 3.246 | 3.311 | 3.272 | 3.261 | 3.248 | 3.258 |
| Mo (229) | 3.142 | 3.112 | 3.162 | 3.130 | 3.119 | 3.114 | 3.116 |
| Rh (225) | 3.786 | 3.756 | 3.832 | 3.782 | 3.756 | 3.749 | 3.764 |
| Pd (225) | 3.876 | 3.839 | 3.942 | 3.875 | 3.855 | 3.828 | 3.864 |
| Ag (225) | 4.070 | 4.001 | 4.148 | 4.053 | 4.013 | 3.990 | 4.021 |
| Ta (229) | 3.298 | 3.252 | 3.320 | 3.281 | 3.231 | 3.242 | 3.244 |
| W (229) | 3.162 | 3.136 | 3.185 | 3.155 | 3.128 | 3.132 | 3.133 |
| Ir (225) | 3.831 | 3.813 | 3.873 | 3.833 | 3.822 | 3.813 | 3.821 |
| Pt (225) | 3.917 | 3.894 | 3.971 | 3.919 | 3.913 | 3.891 | 3.915 |
| Au (225) | 4.067 | 4.048 | 4.161 | 4.084 | 4.078 | 4.045 | 4.077 |
| ME | | -0.071 | 0.056 | -0.005 | 0.018 | -0.036 | -0.024 |
| MAE | | 0.071 | 0.061 | 0.030 | 0.048 | 0.040 | 0.030 |
| MRE | | -1.5 | 1.1 | -0.1 | 0.3 | -0.8 | -0.6 |
| MARE | | 1.5 | 1.2 | 0.6 | 1.1 | 0.9 | 0.7 |

TABLE S2. Bulk modulus $B_0$ (in GPa) of 44 solids. All results were obtained non-self-consistently using PBE orbitals/density. The space group number is indicated in parenthesis.

| Solid | Expt. | LDA | PBE | PBEsol | PBE$u$(PBE) | PBE$u$(PBEsol) | PBE$u$(0.10,0.02) |
|---|---|---|---|---|---|---|---|
| C (227) | 454.7 | 469.8 | 434.7 | 452.1 | 446.4 | 457.0 | 457.2 |
| Si (227) | 101.3 | 95.9 | 88.3 | 93.1 | 93.3 | 94.0 | 94.9 |
| Ge (227) | 79.4 | 71.9 | 59.2 | 67.5 | 70.7 | 70.3 | 72.7 |
| Sn (227) | 42.8 | 45.0 | 36.0 | 41.7 | 47.0 | 44.8 | 47.0 |
| SiC (216) | 229.1 | 230.4 | 212.9 | 221.9 | 218.7 | 222.5 | 225.3 |
| BN (216) | 410.2 | 405.0 | 373.8 | 388.0 | 380.9 | 391.5 | 392.3 |
| BP (216) | 168.0 | 175.8 | 161.9 | 169.5 | 169.3 | 171.3 | 171.8 |
| AlN (216) | 206.0 | 212.2 | 193.9 | 201.9 | 200.3 | 203.6 | 207.0 |
| AlP (216) | 87.4 | 89.9 | 82.5 | 86.7 | 86.4 | 87.6 | 88.3 |
| AlAs (216) | 75.0 | 75.4 | 67.1 | 72.1 | 74.8 | 74.6 | 75.2 |
| GaN (216) | 213.7 | 202.4 | 172.6 | 188.9 | 204.6 | 202.5 | 203.2 |
| GaP (216) | 89.6 | 90.2 | 77.0 | 85.1 | 91.1 | 90.6 | 90.4 |
| GaAs (216) | 76.7 | 73.9 | 60.8 | 69.0 | 75.0 | 74.1 | 74.6 |
| InP (216) | 72.0 | 71.5 | 59.9 | 67.1 | 70.5 | 71.2 | 70.9 |
| InAs (216) | 58.6 | 60.3 | 48.8 | 56.0 | 60.6 | 60.3 | 60.5 |
| InSb (216) | 46.1 | 46.5 | 37.0 | 42.9 | 46.9 | 46.4 | 47.0 |
| LiH (225) | 40.1 | 40.3 | 36.3 | 37.2 | 35.1 | 36.6 | 36.8 |
| LiF (225) | 76.3 | 86.2 | 66.8 | 72.2 | 53.4 | 68.9 | 68.1 |
| LiCl (225) | 38.7 | 40.6 | 31.7 | 35.0 | 31.3 | 37.2 | 33.7 |
| NaF (225) | 53.1 | 61.2 | 44.7 | 48.5 | 43.0 | 51.3 | 51.9 |
| NaCl (225) | 27.6 | 31.7 | 23.6 | 25.6 | 24.0 | 28.3 | 26.6 |
| MgO (225) | 169.8 | 173.1 | 149.3 | 157.8 | 152.8 | 160.9 | 162.5 |
| Li (229) | 13.1 | 15.1 | 13.8 | 13.6 | 13.4 | 13.0 | 13.8 |
| Na (229) | 7.9 | 9.1 | 7.7 | 7.9 | 8.1 | 8.0 | 8.5 |
| Al (225) | 77.1 | 82.4 | 76.5 | 80.9 | 82.9 | 82.3 | 82.9 |
| K (229) | 3.8 | 4.5 | 3.6 | 3.7 | 2.8 | 3.2 | 3.6 |
| Ca (225) | 15.9 | 19.0 | 17.2 | 17.7 | 13.6 | 16.2 | 16.3 |
| Rb (229) | 3.6 | 3.6 | 2.8 | 2.9 | 2.4 | 2.9 | 2.9 |
| Sr (225) | 12.0 | 14.2 | 11.6 | 12.5 | 10.0 | 12.0 | 11.7 |
| Cs (229) | 2.3 | 2.5 | 2.0 | 2.1 | 1.4 | 1.9 | 1.8 |
| Ba (229) | 10.6 | 10.2 | 8.7 | 9.2 | 4.9 | 8.3 | 7.2 |
| V (229) | 165.8 | 209.1 | 181.6 | 196.2 | 215.4 | 213.5 | 211.0 |
| Ni (225) | 192.5 | 256.2 | 197.7 | 230.5 | 215.8 | 244.1 | 232.9 |
| Cu (225) | 144.3 | 191.0 | 142.0 | 169.4 | 138.2 | 175.1 | 161.6 |
| Nb (229) | 173.2 | 190.3 | 168.8 | 181.1 | 182.3 | 188.4 | 185.0 |
| Mo (229) | 276.2 | 291.3 | 257.1 | 278.1 | 286.7 | 289.6 | 288.6 |
| Rh (225) | 277.1 | 318.7 | 257.3 | 295.8 | 317.8 | 328.4 | 307.9 |
| Pd (225) | 187.2 | 228.0 | 169.0 | 205.0 | 210.8 | 236.6 | 206.4 |
| Ag (225) | 105.7 | 139.2 | 90.7 | 119.0 | 132.9 | 142.9 | 131.1 |
| Ta (229) | 202.7 | 215.8 | 192.7 | 205.0 | 233.1 | 221.8 | 223.4 |
| W (229) | 327.5 | 334.0 | 301.0 | 321.3 | 344.7 | 337.8 | 338.7 |
| Ir (225) | 362.2 | 403.5 | 347.6 | 385.1 | 390.9 | 405.6 | 390.4 |
| Pt (225) | 285.5 | 307.6 | 248.2 | 287.7 | 286.1 | 313.3 | 283.2 |
| Au (225) | 182.0 | 193.3 | 137.9 | 173.4 | 174.5 | 196.3 | 174.5 |
| ME | | 10.1 | -11.1 | 0.8 | 2.3 | 7.8 | 4.5 |
| MAE | | 11.6 | 12.2 | 7.8 | 10.3 | 11.7 | 8.5 |
| MRE | | 8.1 | -9.7 | -1.3 | -4.1 | 2.1 | 0.5 |
| MARE | | 9.5 | 10.9 | 6.9 | 11.4 | 8.7 | 7.8 |

TABLE S3. Cohesive energy $E_{\mathrm{coh}}$ (in eV/atom) of 44 solids. All results were obtained non-self-consistently using PBE orbitals/density. The space group number is indicated in parenthesis.

| Solid | Expt. | LDA | PBE | PBEsol | PBE$u$(PBE) | PBE$u$(PBEsol) | PBE$u$(0.10,0.02) |
|---|---|---|---|---|---|---|---|
| C (227) | 7.55 | 8.94 | 7.71 | 8.26 | 7.30 | 7.98 | 7.97 |
| Si (227) | 4.68 | 5.32 | 4.56 | 4.94 | 4.34 | 4.74 | 4.77 |
| Ge (227) | 3.89 | 4.63 | 3.73 | 4.15 | 3.52 | 3.95 | 4.05 |
| Sn (227) | 3.16 | 4.00 | 3.17 | 3.55 | 2.94 | 3.33 | 3.46 |
| SiC (216) | 6.48 | 7.41 | 6.40 | 6.87 | 6.08 | 6.60 | 6.66 |
| BN (216) | 6.76 | 8.04 | 6.93 | 7.40 | 6.12 | 6.90 | 6.95 |
| BP (216) | 5.14 | 6.24 | 5.29 | 5.73 | 5.01 | 5.51 | 5.51 |
| AlN (216) | 5.85 | 6.59 | 5.70 | 6.06 | 4.90 | 5.54 | 5.66 |
| AlP (216) | 4.32 | 4.81 | 4.08 | 4.42 | 3.69 | 4.16 | 4.18 |
| AlAs (216) | 3.82 | 4.47 | 3.68 | 4.04 | 3.25 | 3.76 | 3.81 |
| GaN (216) | 4.55 | 5.40 | 4.40 | 4.83 | 3.97 | 4.47 | 4.57 |
| GaP (216) | 3.61 | 4.34 | 3.49 | 3.89 | 3.39 | 3.77 | 3.77 |
| GaAs (216) | 3.34 | 4.04 | 3.15 | 3.55 | 2.91 | 3.36 | 3.42 |
| InP (216) | 3.47 | 3.96 | 3.14 | 3.53 | 2.84 | 3.32 | 3.32 |
| InAs (216) | 3.08 | 3.74 | 2.89 | 3.27 | 2.48 | 3.01 | 3.07 |
| InSb (216) | 2.81 | 3.45 | 2.63 | 3.00 | 2.31 | 2.76 | 2.86 |
| LiH (225) | 2.49 | 2.67 | 2.35 | 2.44 | 2.14 | 2.35 | 2.39 |
| LiF (225) | 4.46 | 4.92 | 4.33 | 4.48 | 4.43 | 4.59 | 4.65 |
| LiCl (225) | 3.59 | 3.84 | 3.37 | 3.52 | 3.41 | 3.62 | 3.59 |
| NaF (225) | 3.97 | 4.37 | 3.84 | 3.97 | 4.25 | 4.18 | 4.28 |
| NaCl (225) | 3.34 | 3.50 | 3.10 | 3.23 | 3.27 | 3.33 | 3.36 |
| MgO (225) | 5.20 | 5.84 | 4.99 | 5.32 | 5.40 | 5.52 | 5.58 |
| Li (229) | 1.67 | 1.80 | 1.61 | 1.68 | 1.54 | 1.64 | 1.63 |
| Na (229) | 1.12 | 1.24 | 1.08 | 1.15 | 1.16 | 1.16 | 1.15 |
| Al (225) | 3.43 | 4.01 | 3.44 | 3.81 | 3.53 | 3.75 | 3.72 |
| K (229) | 0.94 | 1.01 | 0.87 | 0.93 | 0.88 | 0.91 | 0.89 |
| Ca (225) | 1.87 | 2.20 | 1.91 | 2.11 | 1.94 | 2.12 | 2.00 |
| Rb (229) | 0.86 | 0.92 | 0.77 | 0.84 | 0.83 | 0.84 | 0.81 |
| Sr (225) | 1.73 | 1.88 | 1.61 | 1.81 | 1.78 | 1.88 | 1.76 |
| Cs (229) | 0.81 | 0.88 | 0.72 | 0.78 | 0.68 | 0.75 | 0.70 |
| Ba (229) | 1.91 | 2.24 | 1.88 | 2.12 | 1.69 | 2.10 | 1.85 |
| V (229) | 5.35 | 6.76 | 5.37 | 6.00 | 2.85 | 4.29 | 4.64 |
| Ni (225) | 4.48 | 6.21 | 4.76 | 5.50 | 5.15 | 5.77 | 5.63 |
| Cu (225) | 3.51 | 4.55 | 3.52 | 4.07 | 1.81 | 3.73 | 3.04 |
| Nb (229) | 7.60 | 8.57 | 6.98 | 7.71 | 4.95 | 6.31 | 6.67 |
| Mo (229) | 6.86 | 8.10 | 6.29 | 7.11 | 2.42 | 4.69 | 5.10 |
| Rh (225) | 5.78 | 7.62 | 5.74 | 6.69 | 6.54 | 7.17 | 6.94 |
| Pd (225) | 3.93 | 5.07 | 3.71 | 4.44 | 3.69 | 5.06 | 4.00 |
| Ag (225) | 2.96 | 3.65 | 2.53 | 3.09 | 3.22 | 3.60 | 3.29 |
| Ta (229) | 8.13 | 9.66 | 8.23 | 9.04 | 7.84 | 8.52 | 8.74 |
| W (229) | 8.94 | 10.15 | 8.34 | 9.13 | 4.76 | 6.96 | 7.32 |
| Ir (225) | 6.99 | 9.32 | 7.34 | 8.39 | 7.96 | 8.85 | 8.44 |
| Pt (225) | 5.87 | 7.15 | 5.55 | 6.43 | 6.48 | 7.13 | 6.58 |
| Au (225) | 3.83 | 4.83 | 3.51 | 4.19 | 3.81 | 4.80 | 3.98 |
| ME | | 0.78 | -0.12 | 0.30 | -0.47 | 0.11 | 0.06 |
| MAE | | 0.78 | 0.18 | 0.32 | 0.65 | 0.45 | 0.35 |
| MRE | | 17.5 | -3.7 | 6.4 | -9.3 | 3.3 | 1.3 |
| MARE | | 17.5 | 4.8 | 7.0 | 13.2 | 9.3 | 7.1 |

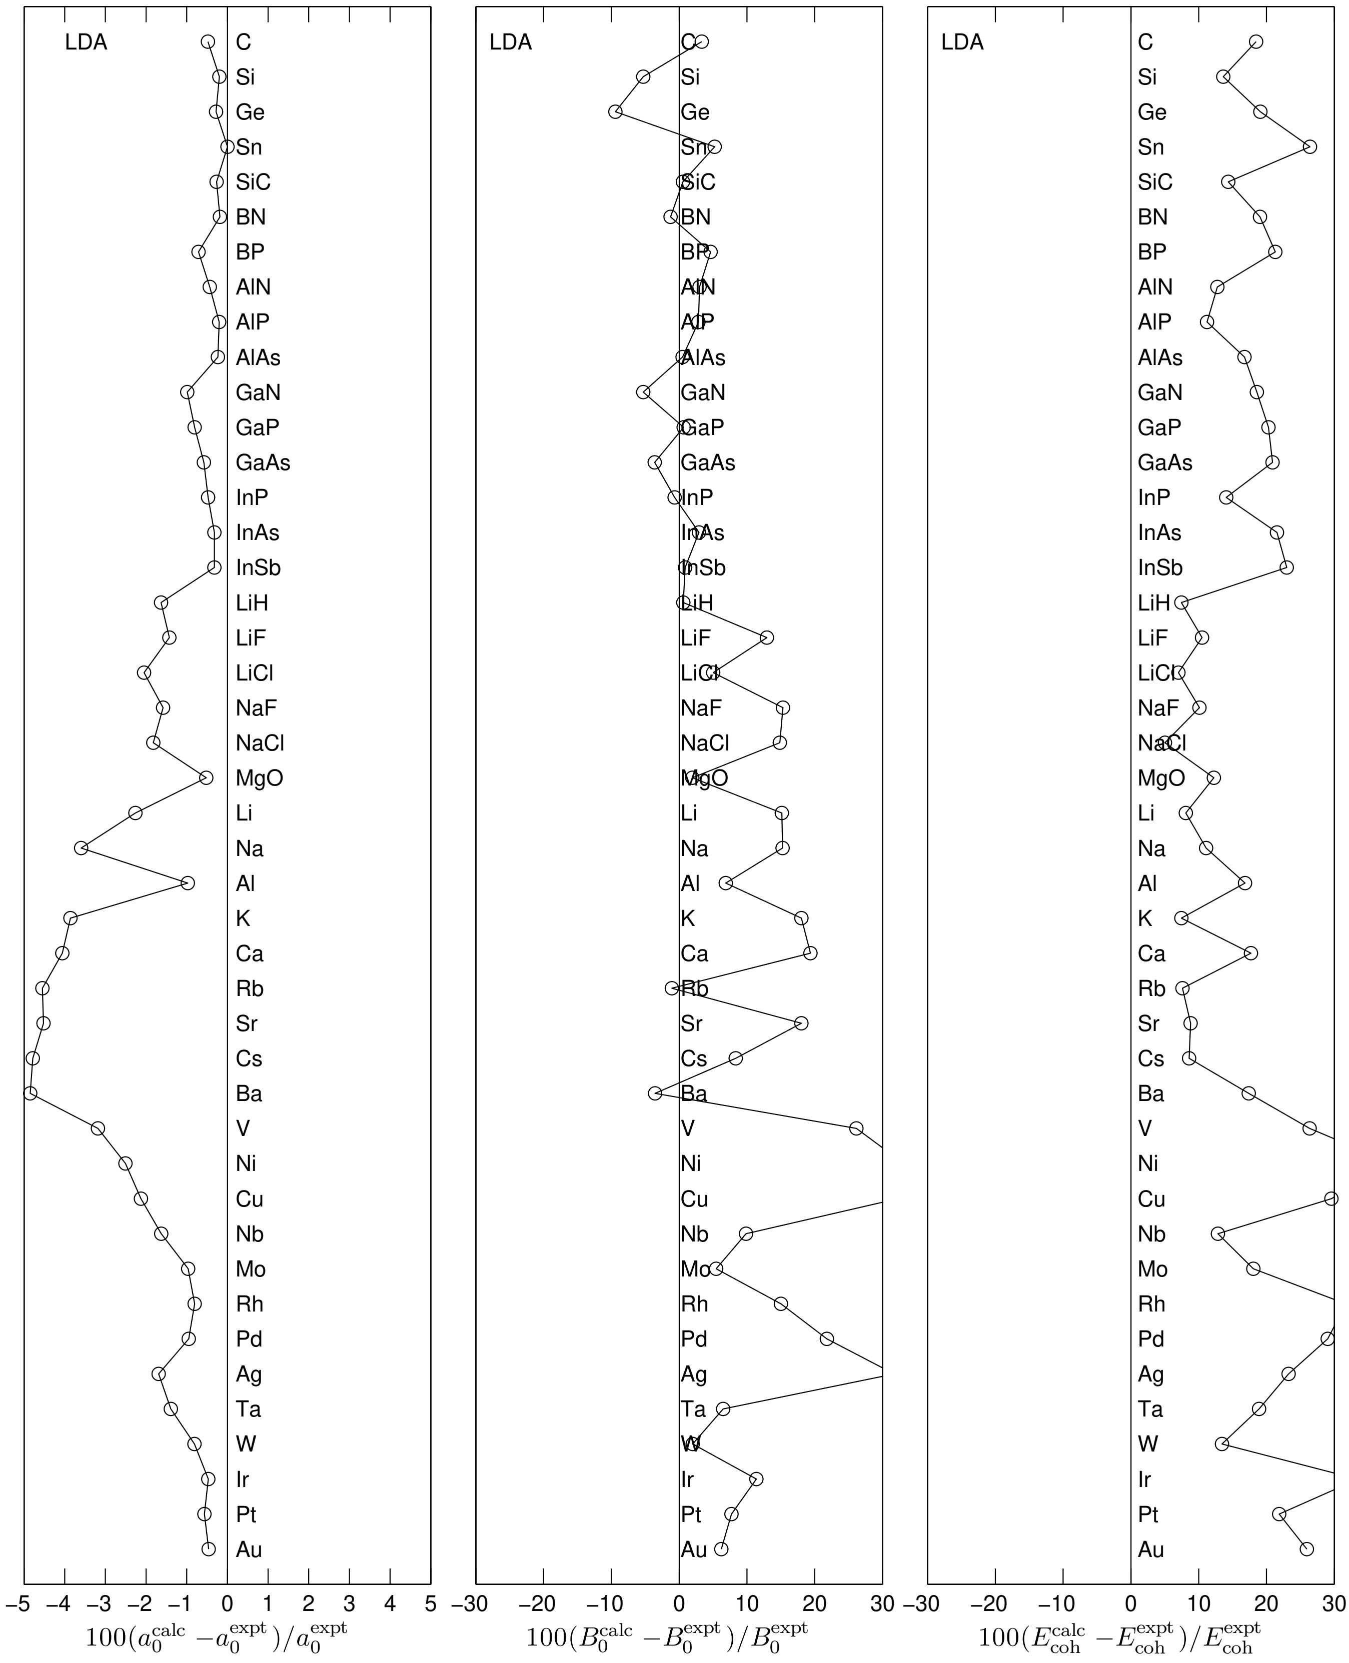


FIG. S1. Relative error (in %) in the calculated lattice constants $a_0$ (left), bulk modulus $B_0$ (middle), and cohesive energy $E_{\rm coh}$ (right) with respect to the experimental values.

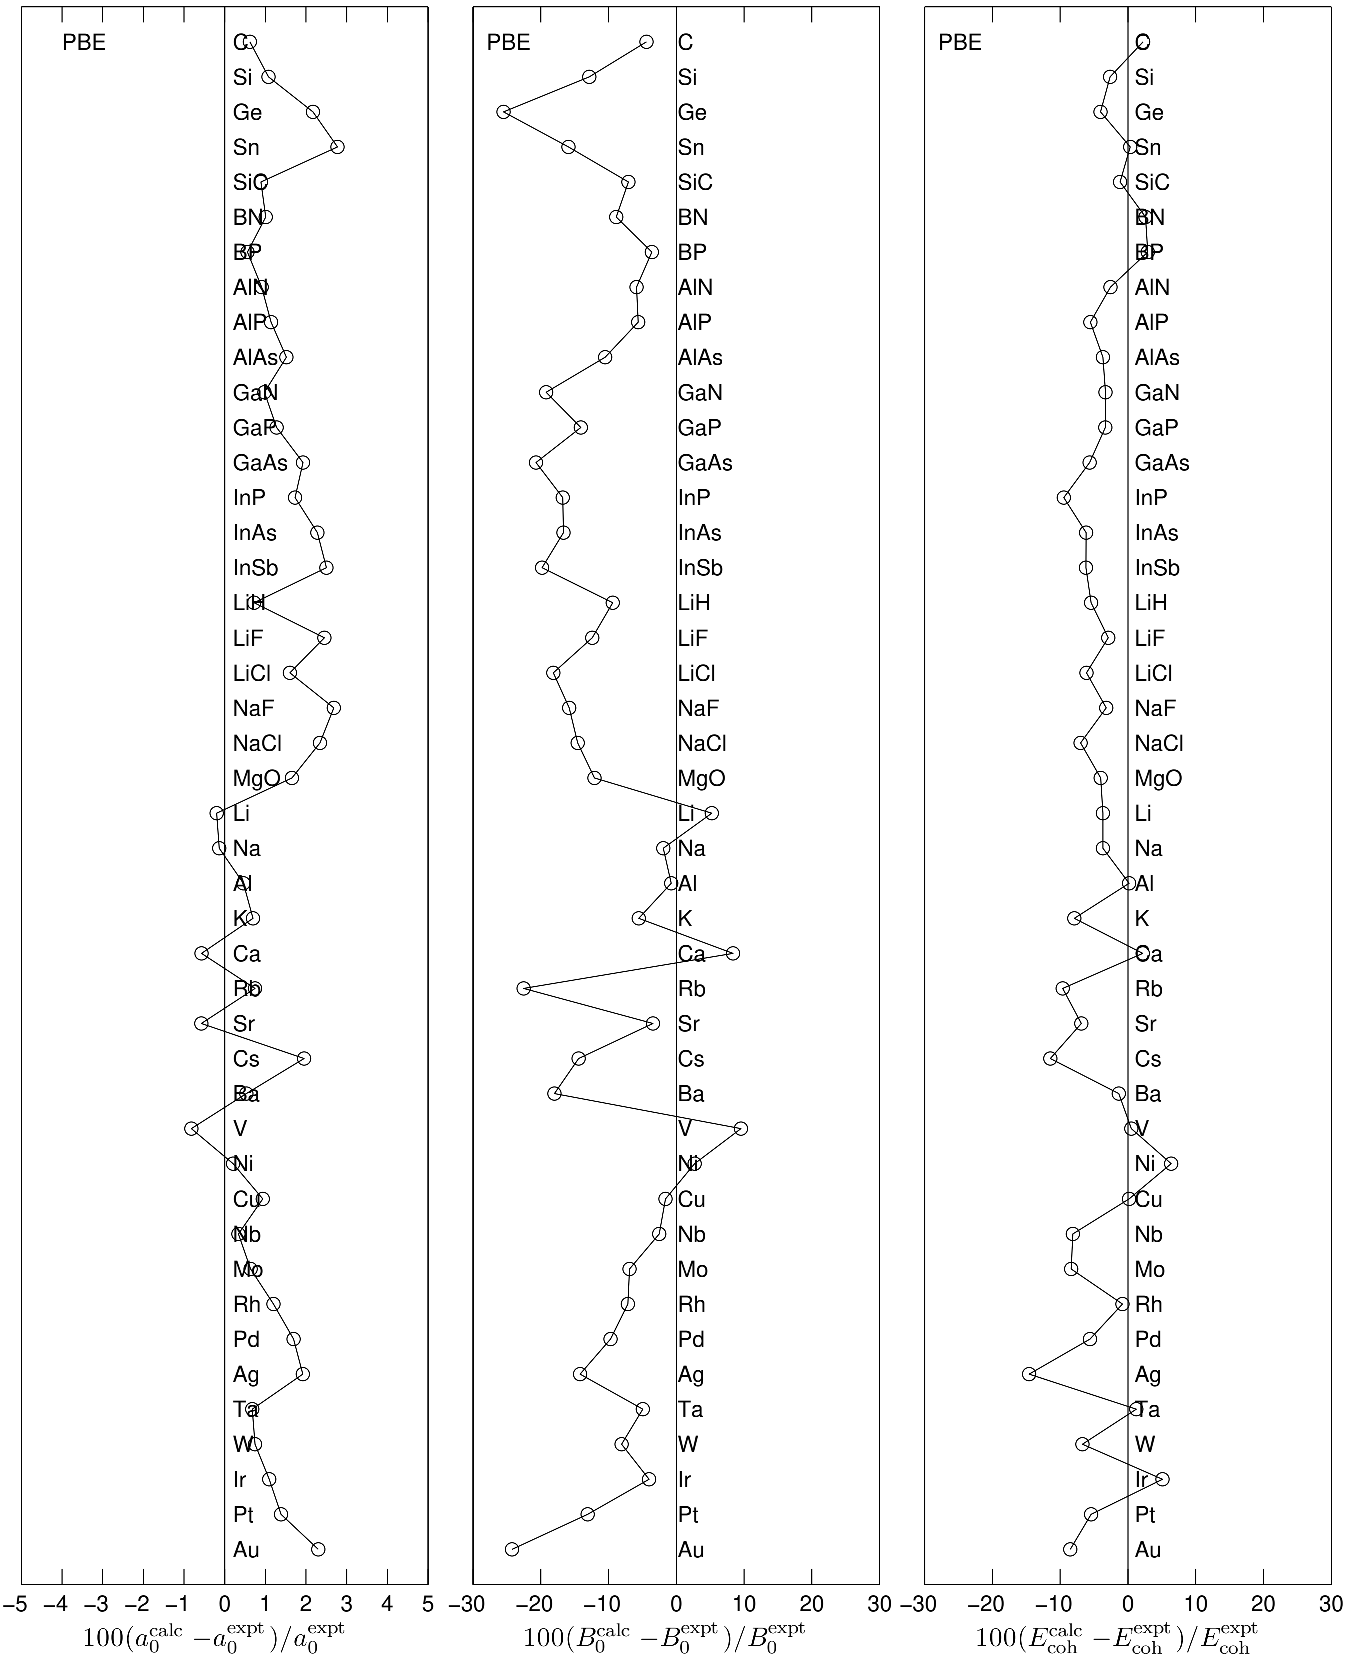


FIG. S2. Relative error (in %) in the calculated lattice constants $a_0$ (left), bulk modulus $B_0$ (middle), and cohesive energy $E_{\rm coh}$ (right) with respect to the experimental values.

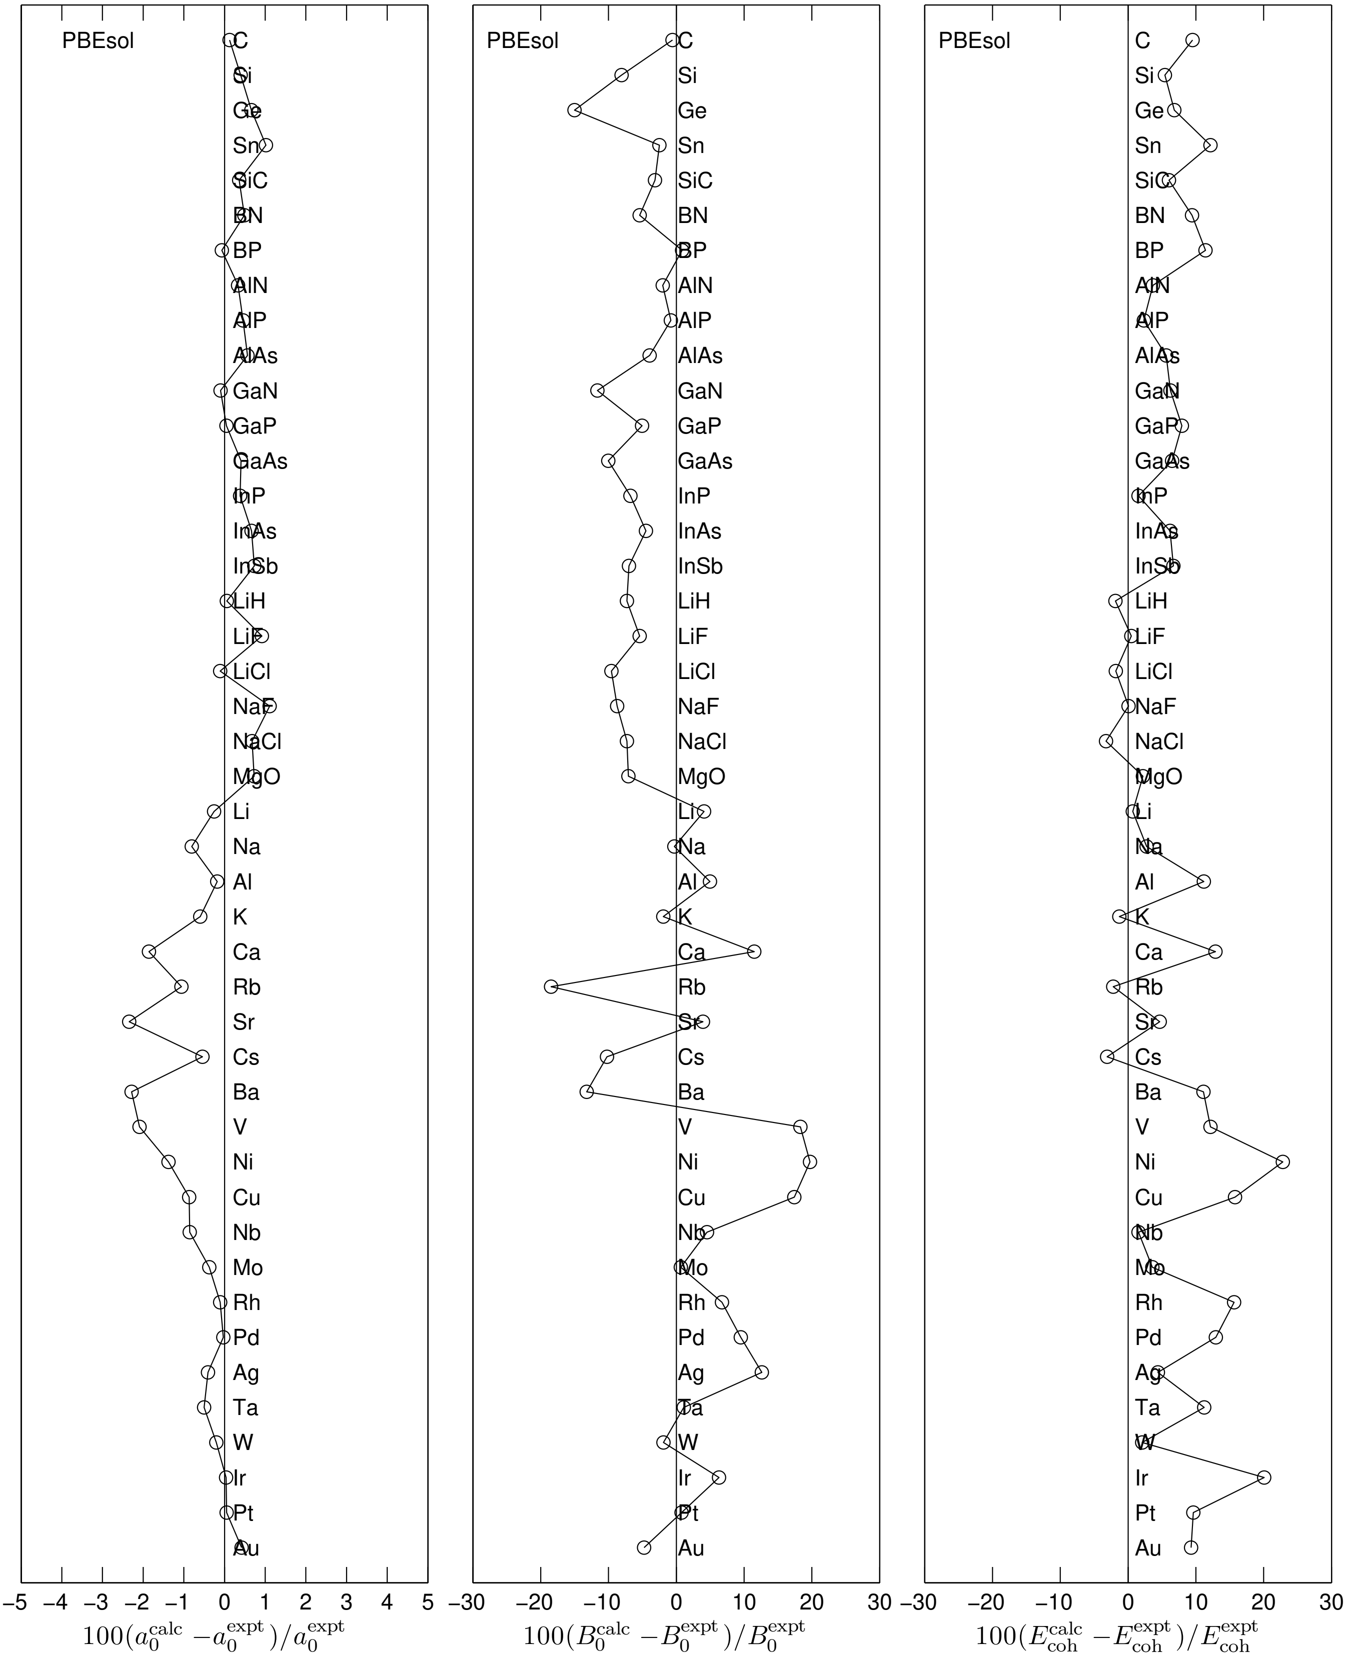


FIG. S3. Relative error (in %) in the calculated lattice constants $a_0$ (left), bulk modulus $B_0$ (middle), and cohesive energy $E_{\rm coh}$ (right) with respect to the experimental values.

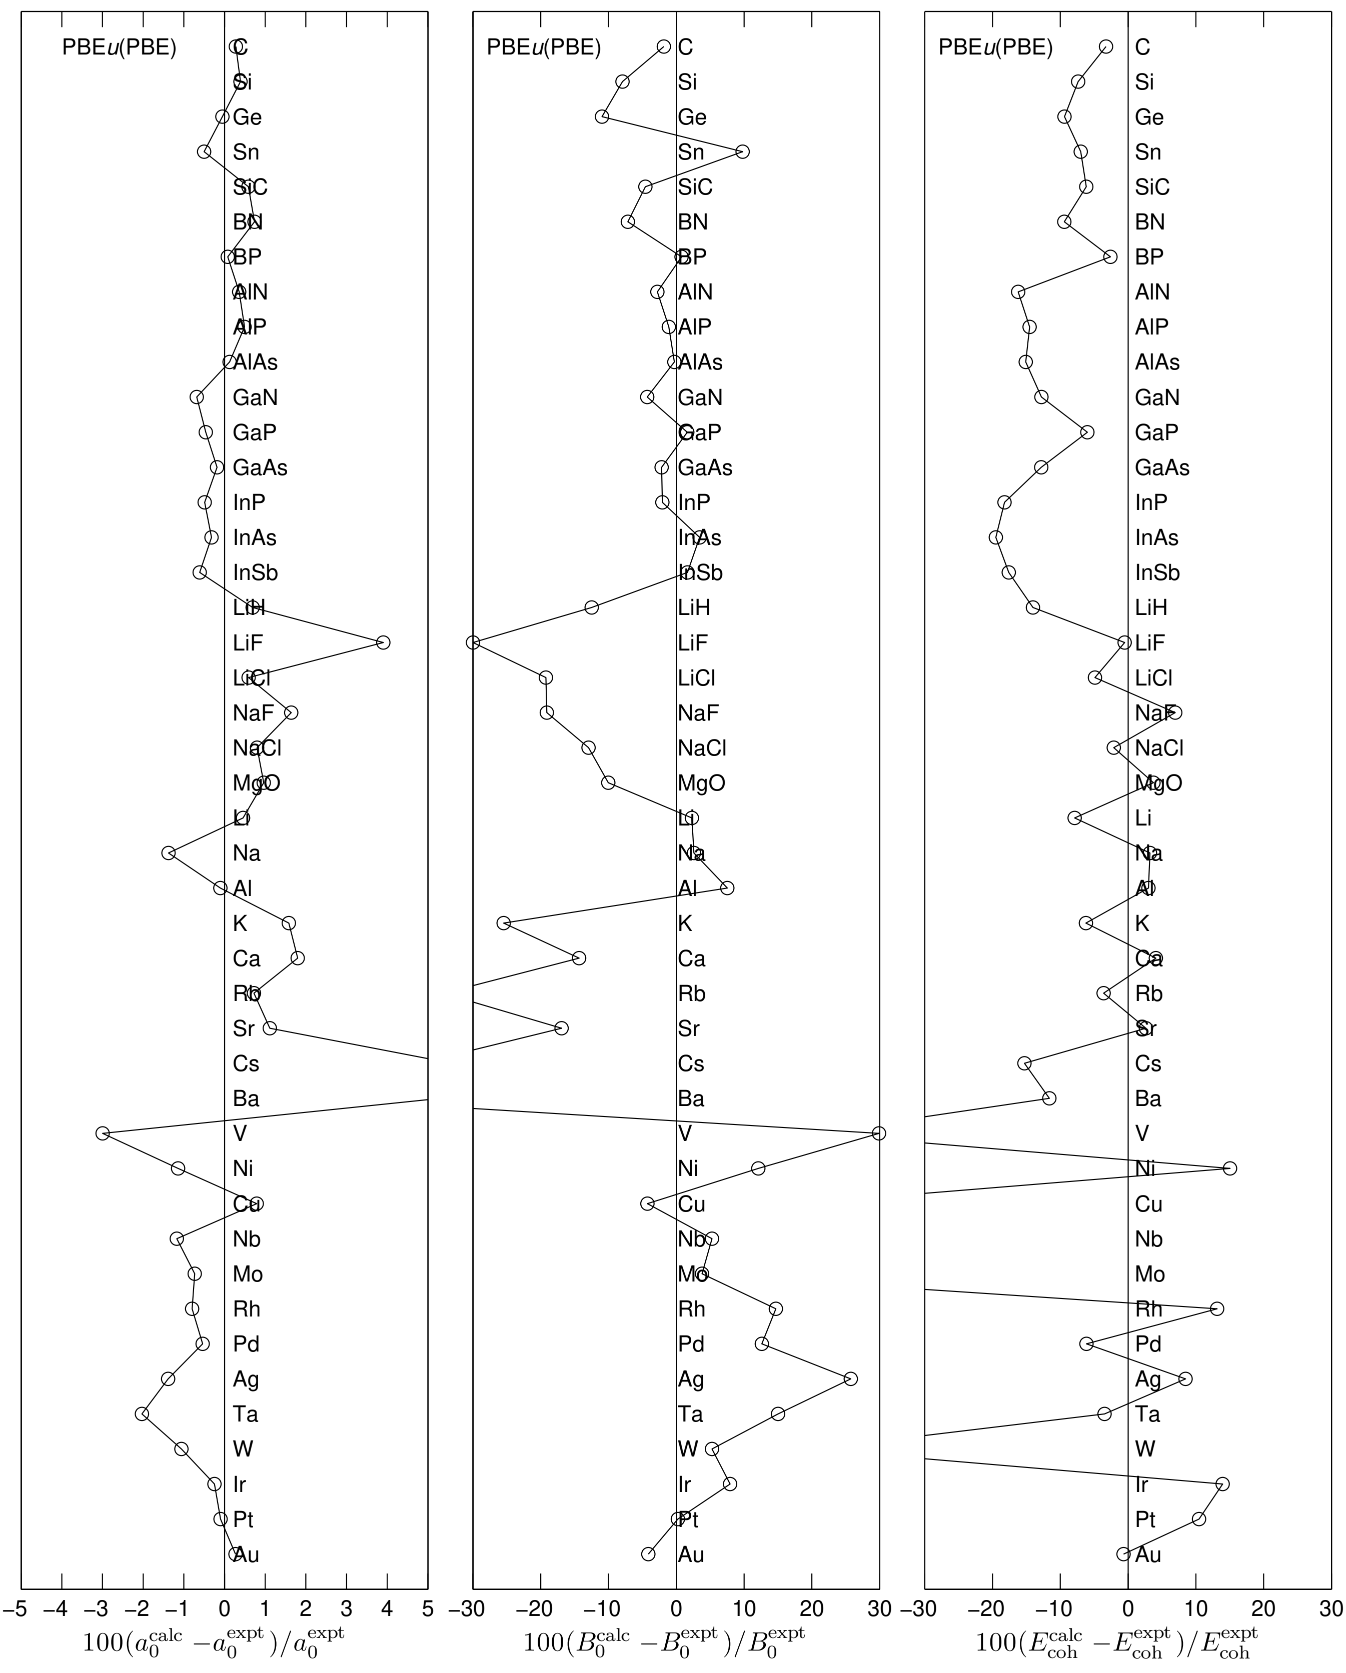


FIG. S4. Relative error (in %) in the calculated lattice constants $a_0$ (left), bulk modulus $B_0$ (middle), and cohesive energy $E_{\mathrm{coh}}$ (right) with respect to the experimental values.

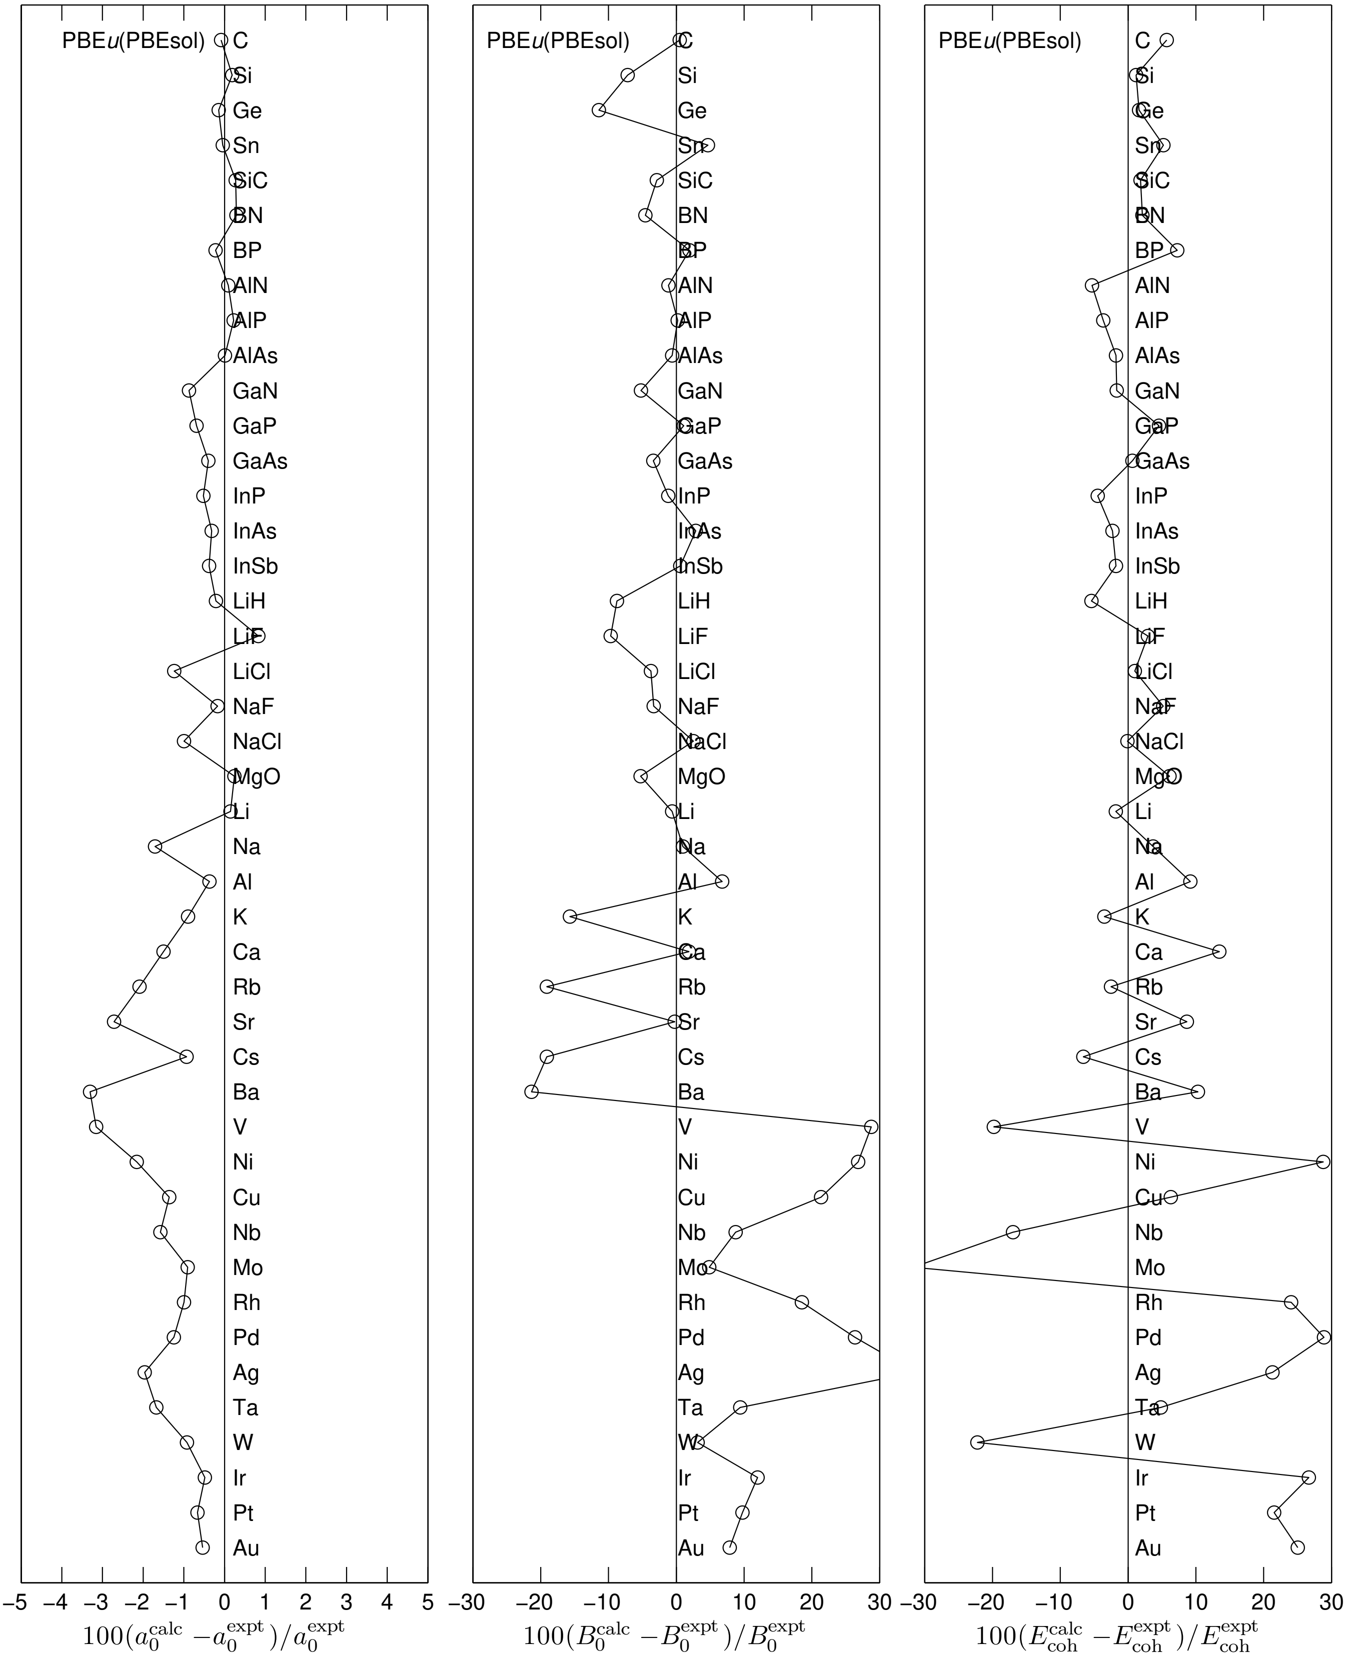


FIG. S5. Relative error (in %) in the calculated lattice constants $a_0$ (left), bulk modulus $B_0$ (middle), and cohesive energy $E_{\rm coh}$ (right) with respect to the experimental values.

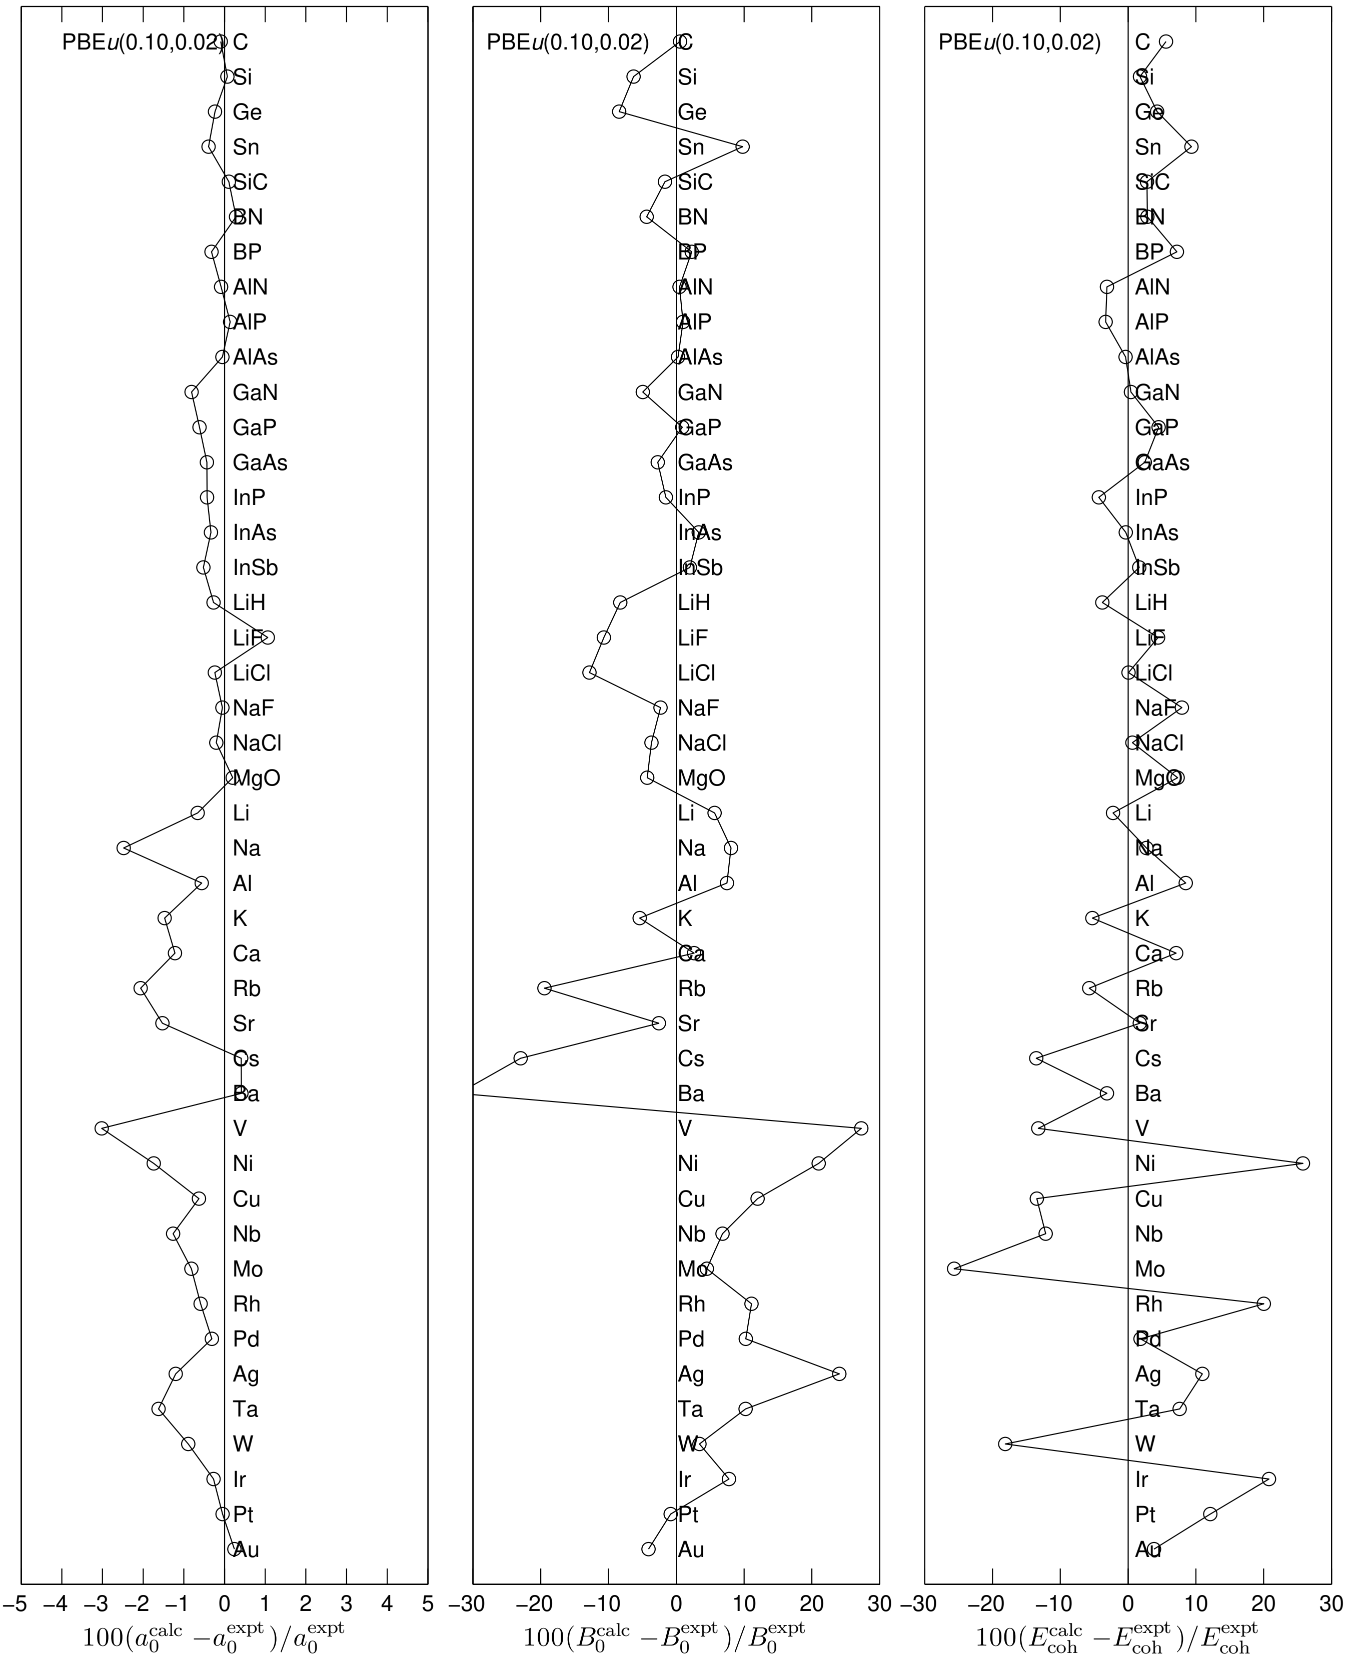


FIG. S6. Relative error (in %) in the calculated lattice constants $a_0$ (left), bulk modulus $B_0$ (middle), and cohesive energy $E_{\rm coh}$ (right) with respect to the experimental values.
